# Supplementary material for: Guaranteed Recovery of One-Hidden-Layer Neural Networks via Cross Entropy
Source: arXiv:1802.06463 source file (2020-05-06)
Supplement: Supplementary file 1 [file supplemental.tex]

\appendices
\input{proof_FCN_classification.tex}
\input{proof_CNN_classification.tex}
%\textbf{\LARGE Supplementary Materials}
\input{proof_initialization.tex}
